# Supplementary material for: A gate-tunable graphene Josephson parametric amplifier
Source: arXiv:2204.02175 ancillary file (2022-04-05)
Supplement: Supplementary file 1 [file g-JPA-arxiv_SI.pdf]

# Supplementary information

## A gate-tunable graphene Josephson parametric amplifier

Guilliam Butseraen,<sup>1</sup> Arpit Ranadive,<sup>1</sup> Nicolas Aparicio,<sup>1</sup> Kazi Rafsanjani Amin,<sup>1</sup> Abhishek Juyal,<sup>1</sup> Martina Esposito,<sup>1</sup> Kenji Watanabe,<sup>2</sup> Takashi Taniguchi,<sup>3</sup> Nicolas Roch,<sup>1</sup> François Lefloch,<sup>4</sup> and Julien Renard<sup>1,\*</sup>

<sup>1</sup>*Univ. Grenoble Alpes, CNRS, Grenoble INP,  
Institut Néel, 38000 Grenoble, France*

<sup>2</sup>*Research Center for Functional Materials,  
National Institute for Materials Science,  
1-1 Namiki, Tsukuba 305-0044, Japan*

<sup>3</sup>*International Center for Materials Nanoarchitectonics,  
National Institute for Materials Science,  
1-1 Namiki, Tsukuba 305-0044, Japan*

<sup>4</sup>*Univ. Grenoble Alpes, CEA, Grenoble INP, IRIG, 38000 Grenoble, France*

## CONTENTS

|                                     |    |
|-------------------------------------|----|
| I. Experimental setups              | 2  |
| II. Device design and fabrication   | 2  |
| III. System charging and time drift | 4  |
| IV. Additional DC measurements      | 6  |
| V. Microwave analysis               | 10 |
| VI. Amplifier Noise analysis        | 15 |
| VII. Additional devices             | 18 |
| References                          | 20 |

---

\* [julien.renard@neel.cnrs.fr](mailto:julien.renard@neel.cnrs.fr)

---

## I. EXPERIMENTAL SETUPS

The results reported in this work were obtained in successive cooldowns in two different dilution refrigerators equipped with dedicated setups. The scheme of the noise measurement setup is shown in Fig. S1a . A shot noise tunnel junction (SNTJ) is used as a calibrated photon source. RF switches allow switching from the graphene Josephson parametric amplifier (JPA) to a  $50\ \Omega$  PCB, making calibration of the gains and losses in the setup possible. The signal is then amplified with a high mobility electron transistor (HEMT), room temperature amplifiers and is measured in a spectrum analyzer. When measuring the noise, the vector network analyzer (VNA) is disconnected and the line is grounded instead. A gate voltage allows to tune the JPA. In this setup, the uncertainty on the microwave power reaching the device was estimated to 3 dB. Data of Figure 4 of the main text were acquired using this setup.

The scheme of the DC measurement setup is shown in Fig. S1b. A lock-in amplifier is used to AC current bias the device (17 Hz) and measure the differential resistance across the graphene Josephson junction (gJJ). A voltage source allows DC biasing of the gJJ and DC voltages are measured with a digital multimeter. The setup can also be used to perform RF measurements with a VNA and an additional pump tone. The 300 K attenuators are changed manually. In this setup, the uncertainty on the microwave power reaching the device was estimated to 4 dB. Data of Figure 1-3 of the main text were acquired using this setup.

## II. DEVICE DESIGN AND FABRICATION

The full geometry of the device is shown in Fig. S2a . The device is made of microstrip lines (Ti/Al 5 nm/60 nm) on a high resistivity Si substrate back-coated with gold. The resonator (purple) has a width of  $10\ \mu\text{m}$  and is coupled to a  $50\ \Omega$  transmission line (red) with a  $5\ \mu\text{m}$  gap (inset 1). Inset 2 shows an optical picture of the center of the device. The width of the resonator locally narrows down at the gJJ location (dimension: width  $w=1.5\ \mu\text{m}$ , length  $l=300\ \text{nm}$ ). We performed AFM on the h-BN/graphene/h-BN stack before making the contacts in order to choose a bubble-free area for the gJJ. Graphene and h-BN flakes are obtained by mechanical exfoliation. We find graphene single layers thanks to optical contrast calibration. The gJJ is gated with a side gate (green) which stops  $500\ \text{nm}$  away from the junction and

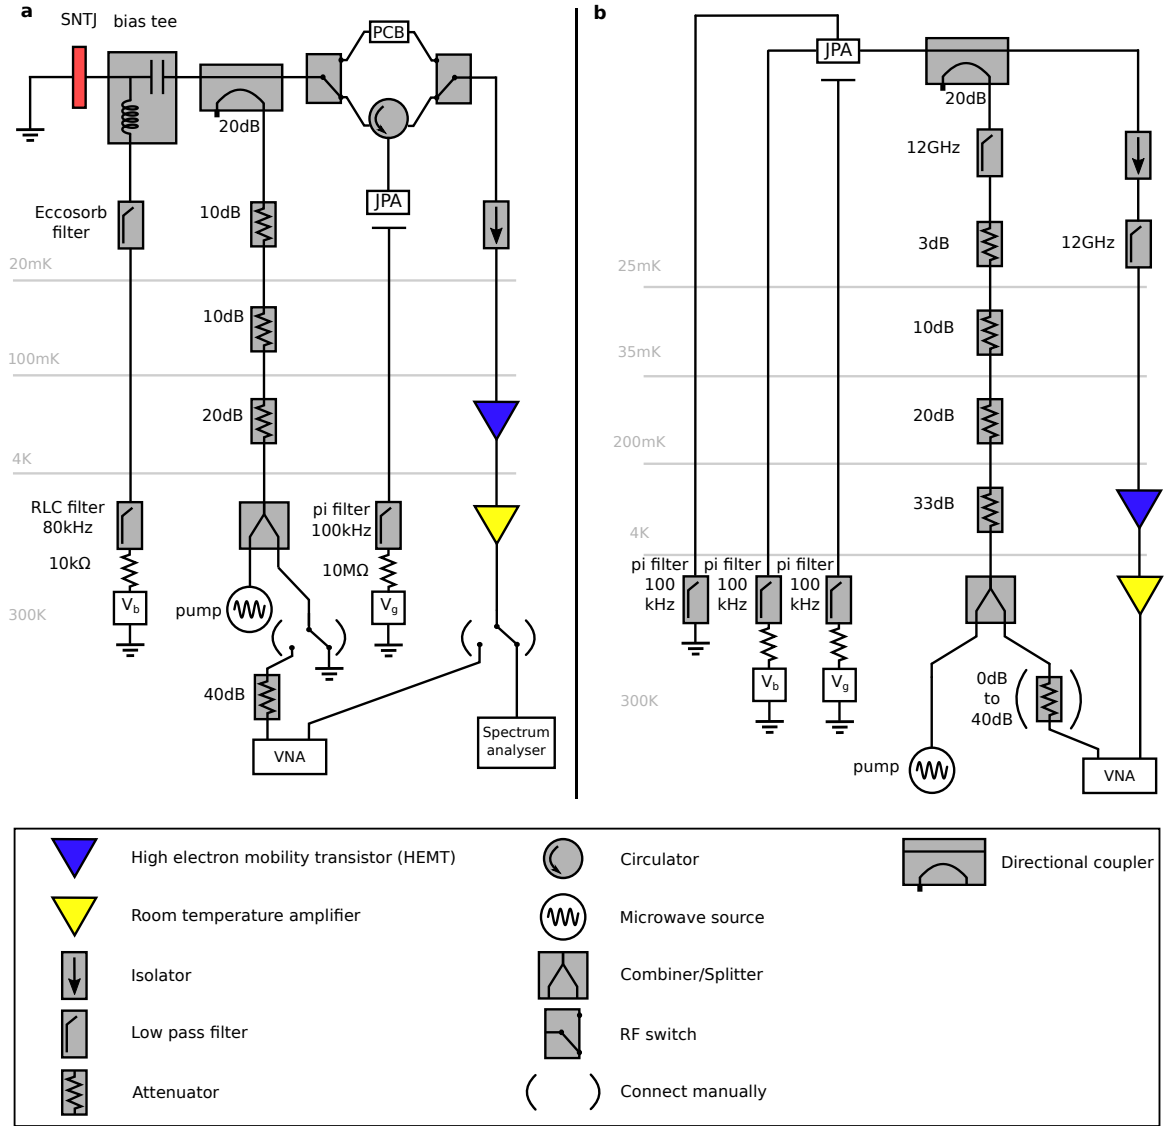

Figure S1: Experimental setups used for noise measurement (a) and DC measurement (b). Both the setups use a dilution fridge and allow for standard microwave measurements.

is extended by an encapsulated graphene part stopping 200 nm away from the gJJ. We designed an on-chip inductor around the bonding pads and Bragg type resonators in order to filter the gating line as well as limiting the coupling with the resonator. We connected the lines used for the DC measurements (blue) very close to the center of the resonator (20  $\mu\text{m}$  away from each side of the gJJ) in order to be at a voltage node, thus having a minimum impact on the resonance. Fig. S2b shows the phase of the measured  $S_{11}$  parameter of the device without a gJJ, and a fit obtained with the circle fit method [1]. We optimized the length and shape of the DC lines such that the parasitic resonances created by adding these lines are above 7 GHz, beyond the

---

maximal working frequency of the device, as shown in Fig. S2b.

### III. SYSTEM CHARGING AND TIME DRIFT

By using the gate on the device, we noticed some effects that we attribute to charge fluctuations and trapping, and also to the use of a side gate. The first noticeable effect is a different behavior when sweeping the gate voltage from positive to negative voltages and the opposite way. In Fig. S3a and b we plot the phase of  $S_{11}$  when sweeping the gate voltage from negative to positive values (a) and positive to negative values (b). We see in Fig. S3a that gating in this direction allows a precise control of the resonance frequency. On the other hand, gating in the other direction (Fig. S3b) shows little effect until an abrupt change around -10 V. All the measurements relying on a gate presented in this article were taken in the configuration of Fig. S3a, i.e. sweeping from negative to positive gate voltages.

The second effect is an evolution of the resonance frequency as function of time after a gate voltage change. In Fig. S3c and d, we plotted the phase of  $S_{11}$  with respect to time for a fixed gate voltage. Fig. S3c was taken right after a gate sweep and Fig. S3d a few minutes later. We see in Fig. S3c a resonance frequency shift of more than 100 MHz in 2 minutes. The shift is faster during the first seconds. In Fig. S3d we see that the drift continues even over hours but on a slower pace. We noticed that the speed of the drift depends on the speed of the gate sweep leading to the gate voltage of interest. In order to limit the effect of this drift and to obtain reproducible datasets, we swept the gate very slowly and waited after each gate change. For gate voltage dependent maps we swept  $V_g$  slowly, for instance in Fig. 1c of the main text, we used the following parameters: a gate voltage step of 0.05 V and a  $S_{11}$  trace time of 75 s for each gate voltage. In Fig. S3e we reproduce Fig. 3b of the main text. The gain is plotted for different gate voltages. We see that for the same gate voltage the amplification frequency can be different. This is explained by the drift mentioned above. We can see for the peaks at 5 V and 15 V, after a long settling time, the final value of the frequency of amplification is different than the initial one. After settling, it matches what is predicted in Fig. S3a: 5.565 GHz at  $V_g = 5$  V and 5.995 GHz at  $V_g = 15$  V, which was measured at a very slow rate of gate voltage change.

In the future, we believe that the use of a top (or bottom) gate should allow to

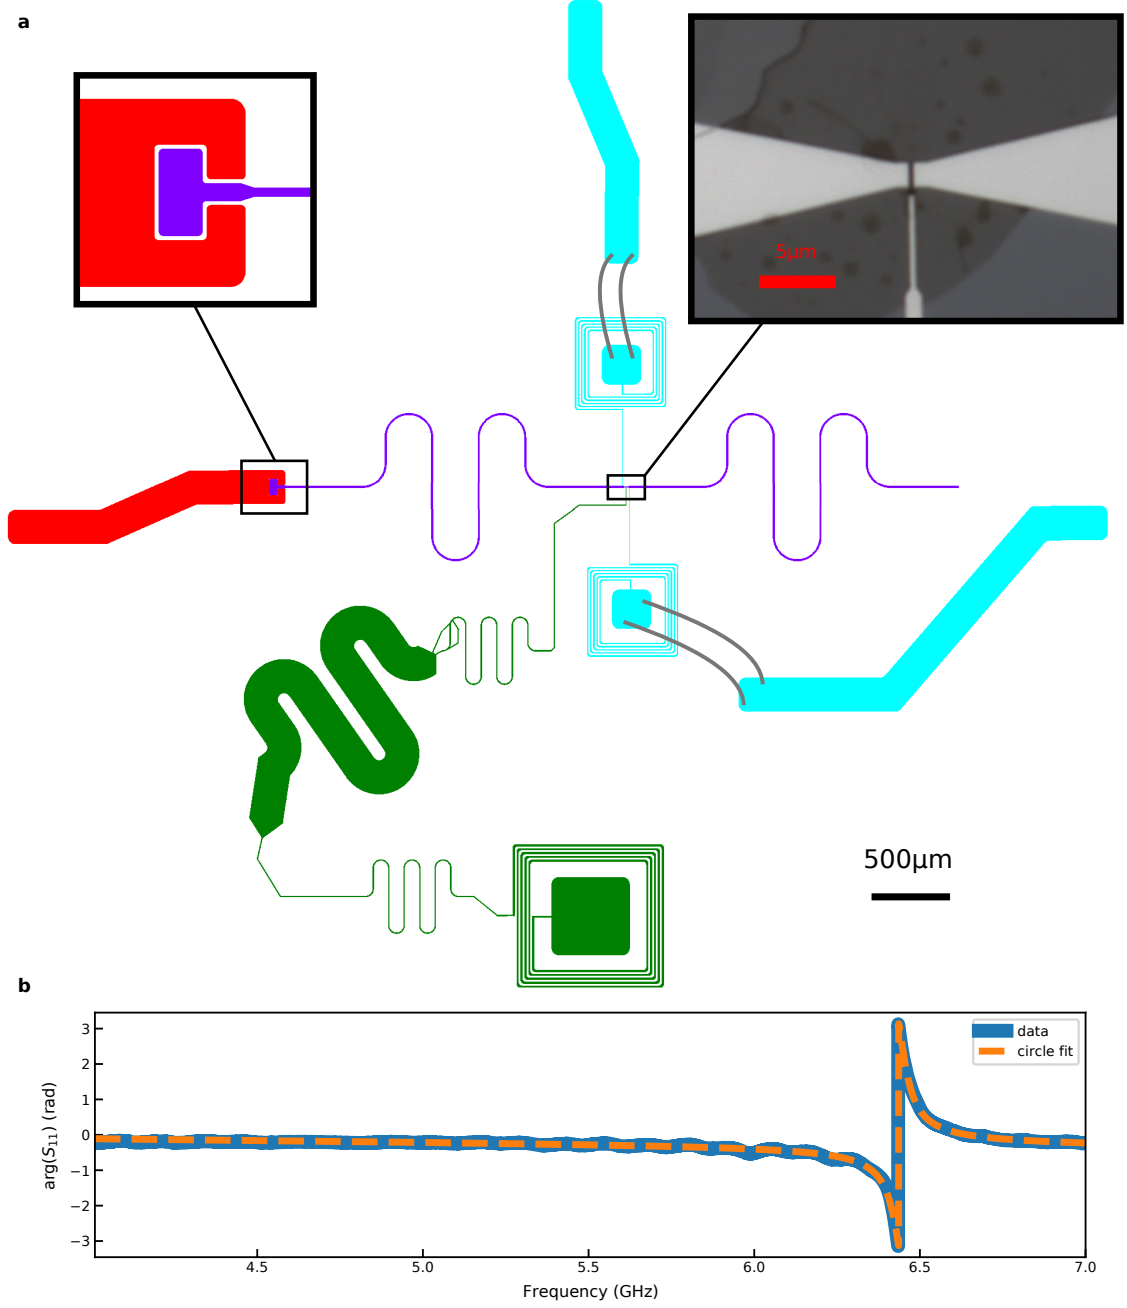

Figure S2: (a) Schematic of the device (to scale). A resonator (purple) is capacitively coupled to a transmission line (red) as shown in the left inset. A side gate (green) is used to tune the gJJ (located in the center of the resonator) critical current. The right inset shows an optical picture of the gJJ. Additional lines (blue) are connected close to the center of the resonator to perform DC measurements on the gJJ. Lines between the pads and the thick lines are bonding wires. (b) Phase of  $S_{11}$  measured and fitted for a bare device where the gJJ is replaced by a short between the two parts of the resonator.

---

suppress those effects. It will indeed be much more efficient than the side gate presented here, allowing the use of smaller voltages, and will be able to screen charges in an efficient manner.

#### IV. ADDITIONAL DC MEASUREMENTS

##### A. Zoom on $\frac{dV}{dI}$

We showed in the main text in Fig. 1b the differential resistance of the device with respect to the gate voltage  $V_g$  and bias current  $I_b$ . Because of the large bias current steps, it is not possible to see fine details. We plot here in Fig. S4, maps that were taken with smaller bias current steps. We see in Fig. S4a that the Dirac point is at  $V_g \approx -3$  V and the minimal critical current is around 100 nA. We also notice oscillations of the critical current that are reminiscent of normal resistance oscillations and are typical in such ballistic junctions [2].

##### B. $R_n I_c$ product

The  $R_n I_c$  product is often used as an indicator of the quality of a Josephson junction. It has been predicted for a short ballistic gJJ without defects:  $e R_n I_c / \Delta \approx 2.4$  where  $\Delta$  is the induced superconducting gap [3]. In order to extract  $\Delta$ , we analyze the differential conductance with respect to the voltage across the gJJ. We extract this bias voltage ( $V_b$ ) using  $dV/dI$  measured with the lock-in amplifier, the integrated resistance measured with a multimeter (Fig. S1b), and the bias current. We show in Fig. S5a the differential conductance with respect to the bias voltage. In a SNS Josephson junction, multiple Andreev reflections (MAR) manifest themselves as peaks in the differential conductance at voltage values equal to  $2\Delta/n$  where  $\Delta$  is the induced superconducting gap and  $n$  integers values [4]. From the  $n=1$  peak we extract an induced gap  $\Delta=147.5$   $\mu$ eV. Fig. S5b shows the normal resistance of the gJJ at 25 mK with respect to the gate voltage measured with a bias current  $I=7$   $\mu$ A such that  $I \gg I_c$ . This enables to plot the  $e R_n I_c / \Delta$  product with respect to the gate voltage in Fig. S5c. We see that the product reaches 1.4 and decreases close to the Dirac point which is generally observed in gJJ [5]. The fact that a side gate is used to change the doping might limit the maximum value of the  $e R_n I_c / \Delta$  product because the charge

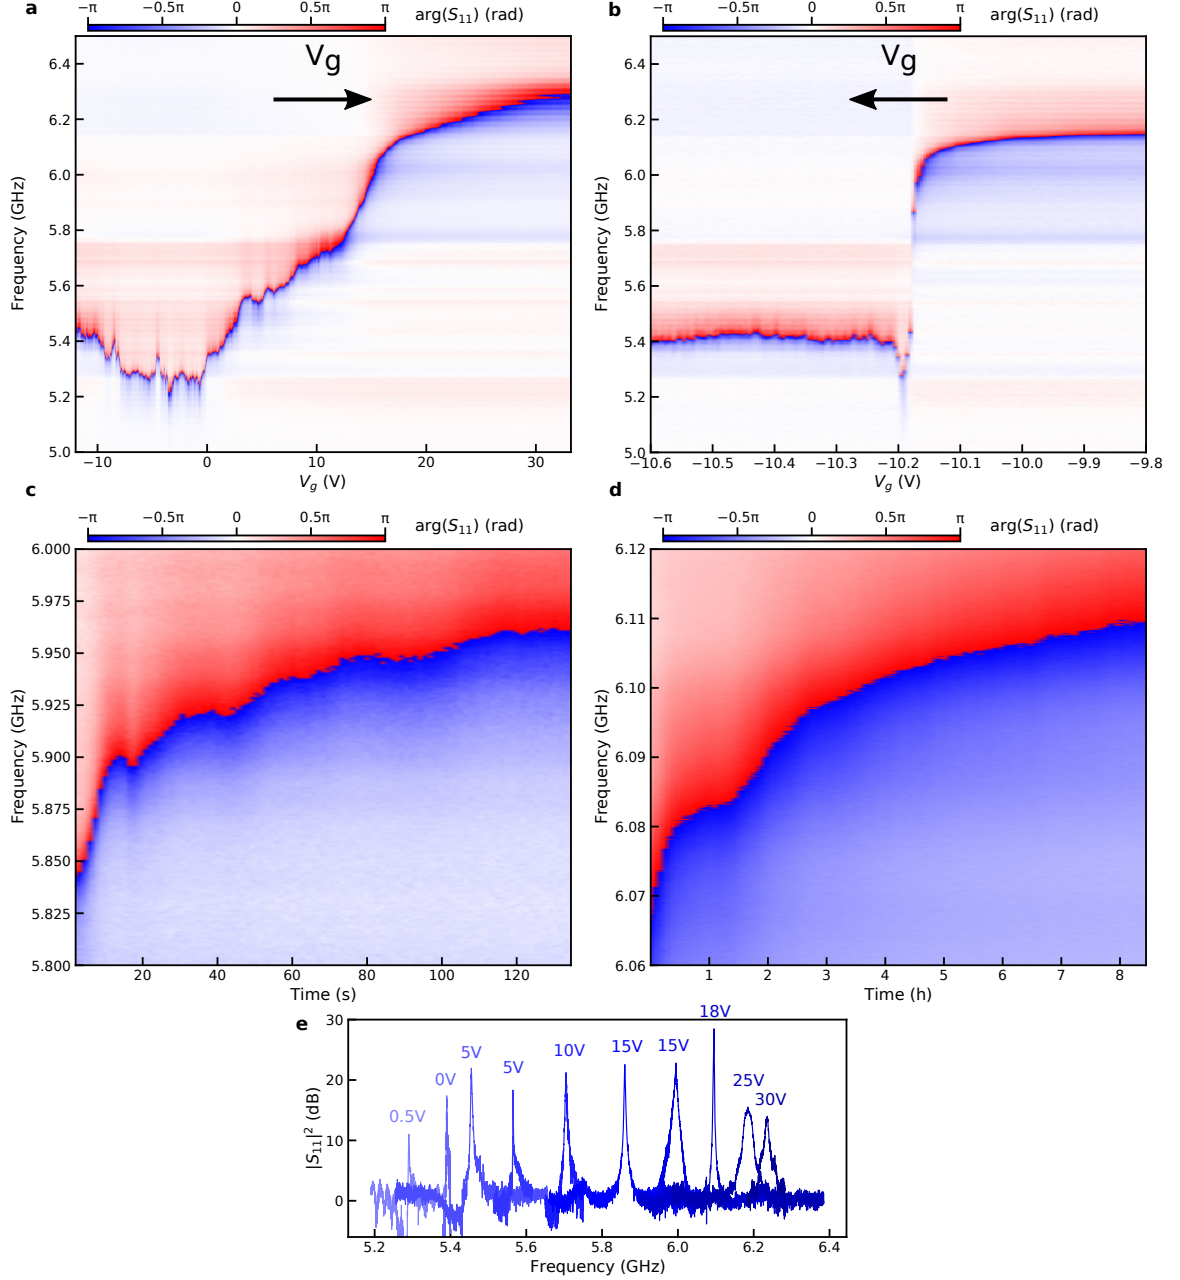

Figure S3: Phase of  $S_{11}$  with respect to the gate voltage when sweeping the gate from negative to positive voltages (a) and positive to negative voltages (b). Phase of  $S_{11}$  with respect to time on a short (c) and a long (d) timescale. (c) is taken right after a voltage sweep from -12 V to 17.5 V with a speed of  $0.17 \text{ V.s}^{-1}$ , (d) is taken a few minutes after (c). (e) Gains obtained at different gate voltages. The system drift explains why at  $V_g = 5 \text{ V}$  and  $V_g = 15 \text{ V}$  it is possible to measure gains at different frequencies.

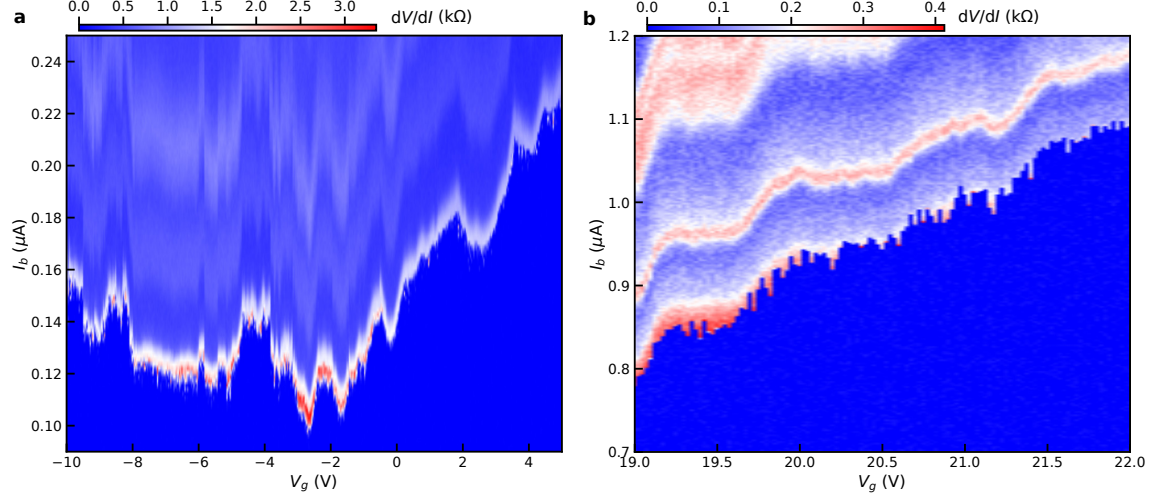

Figure S4: Differential resistance of the graphene Josephson junction with respect to the gate voltage  $V_g$  and bias current  $I_b$  close to the Dirac point (a) and far from the Dirac point (b).

carrier concentration might be non-uniform across the junction.

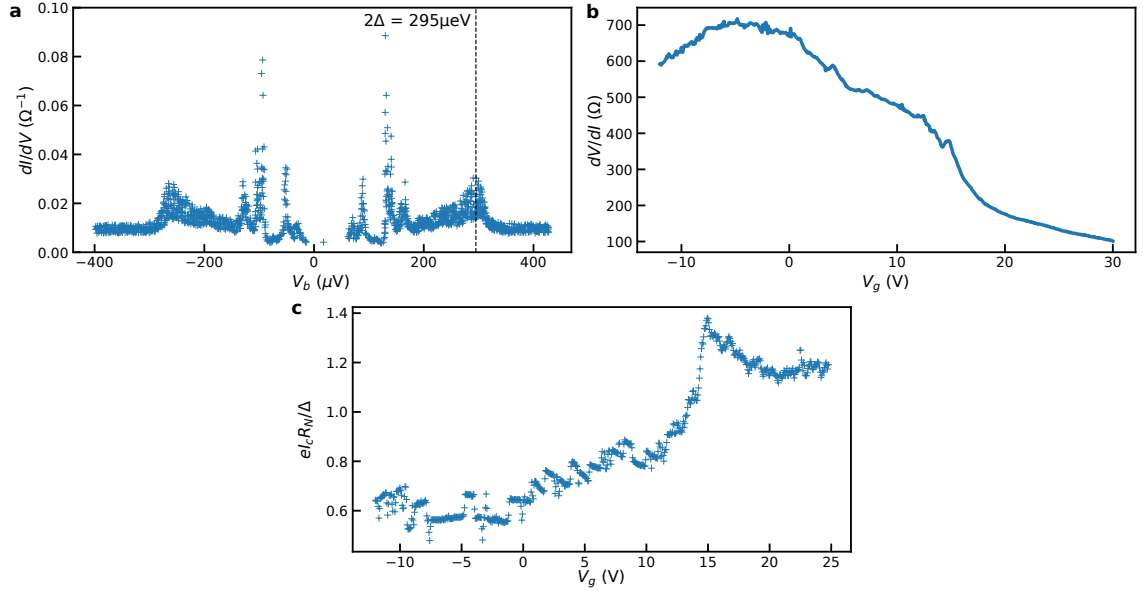

Figure S5: (a) Differential conductance with respect to the gate voltage. The dark line indicates the position of the first MAR peak at a voltage value of  $2\Delta/e$ . (b) Differential resistance as a function of the gate voltage measured at 25 mK with a bias current of 7  $\mu A$ . (c)  $eI_c R_n / \Delta$  product with respect to the gate voltage.

### C. Extracting the Josephson inductance from the critical current

We present here how we obtained Fig. 1d of the main text and why the simple lumped element model is effective to extract  $f_r$ . First, we performed electromagnetic simulations (Sonnet software) replacing the gJJ with a discrete inductance modeling  $L_J$ , the Josephson inductance added by the gJJ. By doing so, we attributed a value of  $L_J$  to each  $f_r$  obtained from  $S_{11}(V_g)$  with the circle fit method. Then, assuming a sinusoidal current phase relation, it is also possible to compute  $L_J$  from the DC measurement of the critical current:

$$L_J = \frac{\phi_0}{2\pi I_c} \quad (1)$$

Fig.S6a shows the comparison between  $L_J$  extracted from RF measurements and DC measurements. At high electron doping,  $L_J$  extracted from RF measurements is higher than what is predicted with a sinusoidal current phase relation (CPR). This indicates a forward skewness of the CPR. Close to the Dirac point, it is the opposite. A backward skewness has never been observed for a gJJ. Therefore we suppose that the measured switching current is smaller than the critical current making the computed  $L_J$  from DC measurements higher than its real value [2].

In a lumped element model, the resonance frequency of the device with a gJJ is  $f_r = 1/(2\pi\sqrt{(L_0 + L_J)C})$  where  $C$  is the equivalent capacitance of the resonator and  $L_0$  the equivalent inductance in the absence of the gJJ. Because we measured a device with the same geometry as the main device presented in this article but without a gJJ, we were able to extract the bare resonance frequency  $f_0 = 1/(2\pi\sqrt{L_0 C})$ . Thus we have the relation:

$$f_r = \sqrt{\frac{L_0}{L_0 + L_J}} f_0 \quad (2)$$

Fig. S6b shows  $f_r$  obtained with *Sonnet* simulations and its fit using Eq.2 with  $L_0$  as a free parameter. By doing so we extract  $L_0=3.9$  nH. We can see that the frequencies obtained by the lumped element model are very close to the frequencies predicted by *Sonnet* simulation with an averaged error of  $\approx 4$  MHz. Therefore this justifies the use of an equivalent lumped element model to compute  $f_r$  with  $L_J$  extracted from DC measurements in the range of experimentally accessible parameters. The error bars in Fig. 1d of the main text are computed by taking only the uncertainty on the critical current that we fixed to  $\Delta I_c=20$  nA being the bias current step used for the

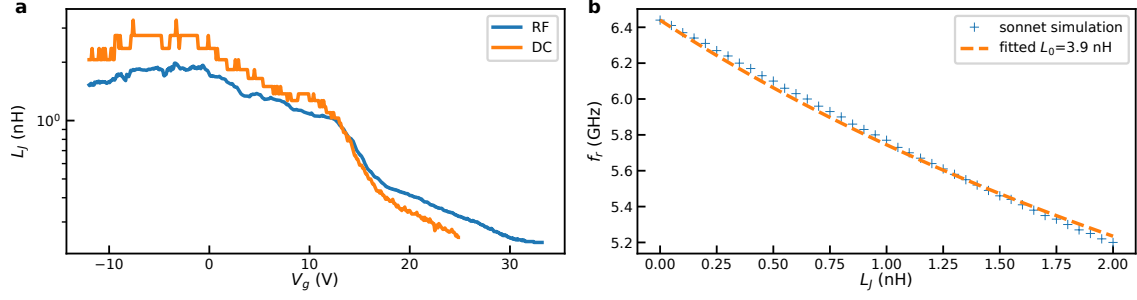

Figure S6: (a) Comparison of the Josephson inductance extracted from RF and DC measurements. (b) Simulated resonance frequencies of the device with *Sonnet* by varying the discrete inductance modeling the Josephson inductance (blue), and its fit with a lumped element model having only  $L_0$  as a free parameter.

measurement. We get from Eq.2 and 1:

$$\Delta f_r = \frac{f_0 \phi_0}{4\pi L_0 I_c^2} \left( 1 + \frac{\phi_0}{2\pi L_0 I_c} \right)^{-\frac{3}{2}} \Delta I_c \quad (3)$$

For low critical currents, we see discrete jumps of the predicted resonance frequency. They are well explained by the biasing current steps of 20 nA being close to  $I_c \approx 100$  nA leading to noticeable jump in  $L_J$  and thus in  $f_r$ .

## V. MICROWAVE ANALYSIS

### A. Two-photon loss model

We used a Kerr based parametric amplifier model in the presence of two-photon loss [6] in order to fit the power dependence of  $S_{11}$  and extract  $\omega_r$ ,  $\gamma_1$ ,  $\gamma_2$ ,  $\gamma_3$  and  $K$ . We also used it to model the gain. In this model, the non linear loss associated with  $\gamma_3$  is proportional to the intra-cavity field power  $|A|^2$ . We can express  $S_{11}$  as:

$$S_{11} = 1 - \frac{2\gamma_1 A}{[i(\omega_r - \omega) + \gamma]A + (iK + \gamma_3)A^3} \quad (4)$$

where  $\gamma = \gamma_1 + \gamma_2$  and  $A$  is the classical intra-cavity field. In order to compute  $A$  we have an additional equation:

$$A^6 + \frac{2[(\omega_r - \omega)K + \gamma\gamma_3]}{K^2 + \gamma_3^2} A^4 + \frac{(\omega_r - \omega)^2 + \gamma^2}{K^2 + \gamma_3^2} A^2 - \frac{2\gamma_1}{K^2 + \gamma_3^2} (b^{in})^2 = 0 \quad (5)$$

where  $b^{in}$  is the classical incoming field. From this equation, we see that the system can have either one real solution or three real solutions (in terms of  $A^2$  because  $S_{11}(A) = S_{11}(-A)$ ). Among the three real solutions, only two are stable. Thus, above a critical power  $(b_c^{in})^2$ , the system bifurcates from a unique state to bi-stable states. This critical power can be computed and expressed as:

$$(b_c^{in})^2 = \frac{4}{3\sqrt{3}} \frac{\gamma^3(K^2 + \gamma_3^2)}{\gamma_1(|K| - \sqrt{3}\gamma_3)^3} \quad (6)$$

### B. Microwave background

Before fitting the  $S_{11}$  parameter with Eq.4, several steps are done in order to correct the microwave background caused by non-ideal elements in the microwave setup (connectors, wirebonds, ...). These elements can cause impedance mismatch creating standing waves in the system. This results in oscillations in the measured  $S_{11}$  making the fit unreliable, especially considering the  $S_{11}$  magnitude on which features are small (typically a few dB).

We first create a normalization trace by averaging  $S_{11}$  measured for different gate voltages (-4.5 V to 18 V) from Fig. 1c of the main text. By doing so, we expect to average out the resonance and obtain the microwave background, i.e. the device independant part. Nevertheless this method has some limitations. First, the resonance width is not negligible ( $\approx 50$  MHz) if we compare it to the full tunability of the device ( $\approx 1$  GHz). The resonance is thus not fully averaged out. Moreover, the gate voltage map has been obtained with a slightly different experimental configuration (i.e. an extra 20 dB room temperature attenuator) compared to the power dependence measurement. Therefore the impedance mismatch is not the same, causing a slightly different microwave background. This method allows nevertheless to reduce significantly the oscillating background down to a level that permits a reliable estimation of the device parameters using a fitting procedure.

### C. Fitting method

Because of the large numbers of free parameters it was not possible to fit directly  $S_{11}$ . We tried to use the circle fit method at a low input power  $P_0$  to obtain  $\omega_r$ ,  $\gamma_1$ ,

$\gamma_2$  [1]. Nevertheless, the fitted  $\omega_r$ ,  $\gamma_1$  and  $\gamma_2$  were not compatible with the measured value of  $\Delta\omega = \omega_c - \omega_r$  where  $\omega_c$  is the frequency at which the electromagnetic field is maximum in the device at the critical power (i.e. frequency at which the depth of  $|S_{11}|$  is minimum):

$$\Delta\omega = -\gamma \frac{K}{|K|} \left[ \frac{4\gamma_3|K| + \sqrt{3}(K^2 + \gamma_3^2)}{K^2 - 3\gamma_3^2} \right] \approx -\sqrt{3}\gamma \frac{K}{|K|} \quad (7)$$

We can make the last approximation when  $\gamma_3 \ll K$  which is the case here. Several reasons can explain the fact that this fitting method is unreliable. First, as we already mentioned the microwave background was not totally canceled out by the normalization method. Moreover, the two-photon loss model only takes into account the quartic nonlinear term in the development of the current phase relation. It has been shown that taking the full development has an impact on  $\Delta\omega$  [7]. In a gJJ, the current phase relation is not exactly sinusoidal which makes the model less accurate. Last, the losses are not always increasing linearly with the input power depending on the gate voltage. So, the two-photon loss model is not describing the system perfectly, but we used it as an approximation because developing a more complete model was beyond the scope of this work.

To get rid of the microwave background, we used the lowest input power  $S_{11}(P = P_0)$  trace ( $b_c^{in} \ll b_c^{in}$ ) as a normalization trace. We then fixed  $\gamma_2$  as a function of  $\gamma_1$  using Eq.7 by taking the experimentally determined  $\Delta\omega$ . We fixed  $b_c^{in}$  by manually finding the input power at which the system bifurcates (power at which we see an infinite derivative of  $S_{11}$ ). We then fitted  $S_{11}(P = P_c)$  at the critical power normalized by  $S_{11}(P = P_0)$  with only two free parameters:  $\gamma_1$  and  $\gamma_3$  by calculating  $K$  with Eq.6 and taking  $\omega_r$  extracted with the circle fit method. At  $P = P_0$ , there is a slight frequency shift compared to the limit  $P = 0$  where the nonlinear effects are fully absent. Therefore, we shift  $\omega_r$  accordingly to match the experimental resonance frequency at this power. Because we modified  $\omega_r$ , we changed  $\Delta\omega$  accordingly ( $\Delta\omega = \omega_c - \omega_r$ ). Having a new  $\Delta\omega$ , we finally fitted  $|S_{11}(P = P_c)/S_{11}(P = P_0)|$  with only  $\gamma_1$  and  $\gamma_3$  as free parameters and  $K$  computed with Eq.6.

Fig. S7a and b show the result of this fitting method for two different working frequencies at input powers  $P_c$  and  $P_0$ . We see good agreements between the fit and the data. By fitting  $S_{11}$  at the critical power, we get all the parameters needed to fit

$S_{11}$  at any power. Fig. S7c and d show the amplitude of  $S_{11}$  at different input powers  $P$  normalized by the amplitude of  $S_{11}$  at low input power  $P_0$ . This helps to get rid of the microwave background and shows the evolution of the losses with the power. For  $f_r \approx 5.85$  GHz, we see that the depth of the peak is well described by the two-photon loss model: losses are increasing linearly with the power. But for  $f_r \approx 6.17$  GHz, we see that the two-photon loss model does not describe the losses correctly. Indeed, the depth of the resonance is not increasing linearly with the power: higher orders of losses are needed to describe the system. In this case, because we obtained  $\gamma_3$  by fitting the losses at the critical power (purple), we thus overestimated the losses at lower powers.

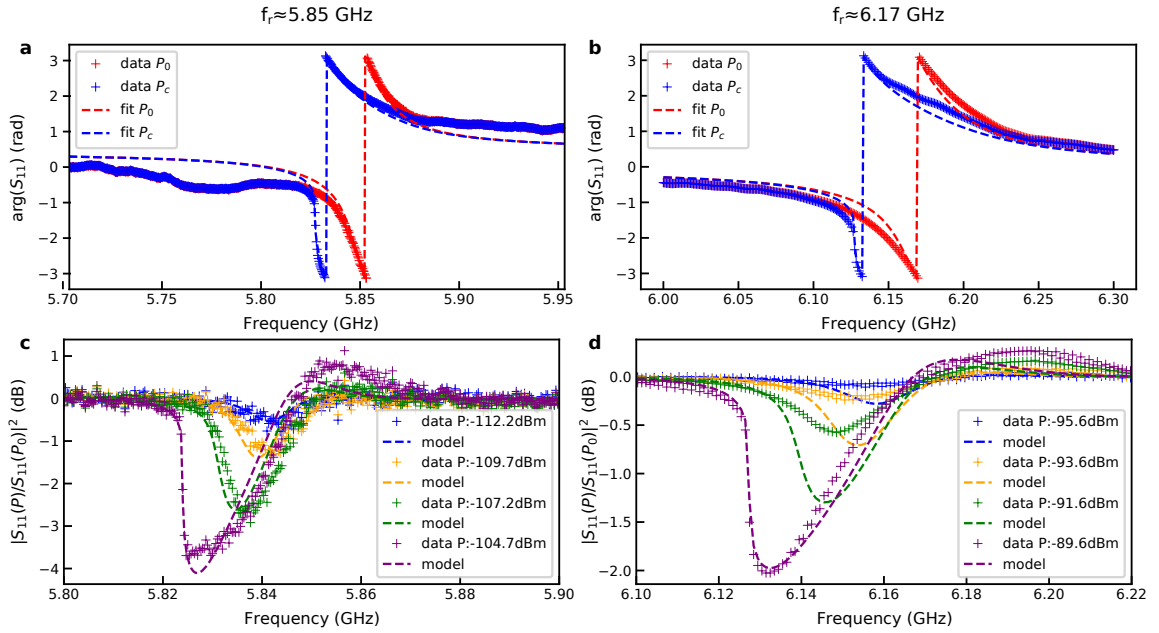

Figure S7: (a) and (b): Phase of  $S_{11}$  at low input power  $P_0$  and critical input power  $P_c$  for two working frequencies. The fits are obtained by the fitting method described in Sec. VC. (c) and (d): Amplitude of  $S_{11}$  at various input power normalized by the amplitude of  $S_{11}$  at input power  $P_0$  for two working frequencies. The critical power is showed in purple.

#### D. Modeling the gain

The two-photon loss model does not include saturation effect mechanisms (except for the nonlinear loss itself that can reduce the amplification), leading to a possible infinite gain when the optimal pump power and frequency are chosen. Experimentally, JPAs exhibit saturation of the gain, mainly because of higher order non linear terms

in the expansion of the current phase relation, shifting  $\omega_c$  and therefore putting the pump out of resonance [7]. We did not build a model with the full development of the current phase relation with two-photon loss. Instead, we adopted a phenomenological approach using the two-photon loss model. In this model the gain can be expressed as:

$$G = \frac{|(-i\omega + \lambda_0)(-i\omega + \lambda_1) - 2\gamma_1(-i\omega + W^*)|^2}{(\omega^2 + \lambda_0^2)(\omega^2 + \lambda_1^2)} \quad (8)$$

with:

$$\lambda_0 = \gamma + 2\gamma_3 A^2 - \sqrt{(K^2 + \gamma_3^2)A^4 - (\omega_r - \omega_p + 2KA^2)^2} \quad (9)$$

$$\lambda_1 = \gamma + 2\gamma_3 A^2 + \sqrt{(K^2 + \gamma_3^2)A^4 - (\omega_r - \omega_p + 2KA^2)^2} \quad (10)$$

$$W = i(\omega_r - \omega_p) + \gamma + 2(iK + \gamma_3)A^2 \quad (11)$$

$\omega_p$  being the pump pulsation and  $\omega$  the signal pulsation. The pump pulsation and power are fixed by the experiment. We then considered the pump power being at  $0.95b_c^{in}$ . All the other parameters are obtained with the previous fit method of  $S_{11}$  at the critical power where  $K$  is adjusted to match the new critical power with Eq.6. In order to reproduce the shift in frequency happening because of higher order non-linear terms, we corrected  $\omega_r$  until we find the maximum gain corresponding to the measurement.

### E. Parameters for the simulations of the main text

Table S1: Parameters for the simulation in Fig. 2b of the main text

| $\omega_r$ (rad.s <sup>-1</sup> ) | $\gamma_1$ (rad.s <sup>-1</sup> ) | $\gamma_2$ (rad.s <sup>-1</sup> ) | $\gamma_3$ (rad.s <sup>-1</sup> ) | $K$ (rad.s <sup>-1</sup> ) | $b_c^{in}$ (Hz <sup>0.5</sup> ) |
|-----------------------------------|-----------------------------------|-----------------------------------|-----------------------------------|----------------------------|---------------------------------|
| 36 751 325 120                    | 68 989 805                        | 5 980 569                         | 68 866                            | -847 738                   | 93 802                          |

Table S2: Parameters for the simulation of the gain in Fig. 3a of the main text

| $\omega_r$ (rad.s <sup>-1</sup> ) | $\gamma_1$ (rad.s <sup>-1</sup> ) | $\gamma_2$ (rad.s <sup>-1</sup> ) | $\gamma_3$ (rad.s <sup>-1</sup> ) | $K$ (rad.s <sup>-1</sup> ) | $b_c^{in}$ (Hz <sup>0.5</sup> ) |
|-----------------------------------|-----------------------------------|-----------------------------------|-----------------------------------|----------------------------|---------------------------------|
| 36 975 339 700                    | 68 989 805                        | 5 980 569                         | 68 866                            | -696 892                   | 103 914                         |

## VI. AMPLIFIER NOISE ANALYSIS

### A. Noise fitting formula

We used a SNTJ as a broadband noise source in order to extract the added noise by the whole amplification chain. We can model the power spectral density  $N$  measured at the spectrum analyzer plane by:

$$N = B[G_{ss}(N_s + N_{int}) + G_{si}N_i] \quad (12)$$

where  $B$  is the bandwidth of the spectrum analyzer,  $G_{ss}$  is the total gain at the signal frequency  $f_s$ ,  $G_{si}$  the conversion gain from the idler to the signal frequency,  $N_s$  the power spectral density emitted by the SNTJ at the signal frequency,  $N_i$  the power spectral density emitted by the SNTJ at the idler frequency  $f_i = 2f_{pump} - f_s$ , and  $N_{int}$  the intrinsic noise added by the whole chain. We had to consider the conversion from idler to signal frequency because the SNTJ is a broadband noise source [8, 9].  $N_{int}$  is dominated by the first element of the amplification chain. For example, if we consider only the JPA and the HEMT, we have  $N_{int} = N_{JPA} + N_{HEMT}/G_{JPA} \approx N_{JPA}$  if  $G_{JPA}$ , the gain of the JPA, is high enough. At high gain we can make the approximation  $G = G_{ss} = G_{si}$  which shows that the total noise added by the system is:  $N_{int} + N_i$  where  $N_i = hf_s/2$  when there are only quantum fluctuations in the idler channel. Thus, at best, if there is no intrinsic noise coming from the JPA, the minimal added noise is half a photon coming from the idler channel: this is the standard quantum limit (SQL). We plotted in Fig. 4 of the main text the total noise added by the system  $N_{int} + N_i$  with  $N_i = hf_s/2$ .

We can express the noise power emitted by the SNTJ as:

$$N(f) = \frac{1}{2} \left[ \left( \frac{e(V - V_{shift}) + hf}{2} \right) \coth \left( \frac{e(V - V_{shift}) + hf}{2k_B T} \right) + \left( \frac{e(V - V_{shift}) - hf}{2} \right) \coth \left( \frac{e(V - V_{shift}) - hf}{2k_B T} \right) \right] \quad (13)$$

where  $T$  is the electronic temperature of the SNTJ,  $V$  the bias voltage of the SNTJ and  $V_{shift}$  an offset voltage. We can separate the gain contribution of the JPA and the rest of the chain such that  $G_{ss} = G_{chain}G_{JPA,ss}$ . We made the approximation  $G_{JPA,si} = G_{JPA,ss} - 1$  which is exact if there is no intrinsic loss in the JPA, and we

simplify the notation:  $G_{JPA,ss} = G_{JPA}$ . Eq.12 gives:

$$N = BG_{chain} \left[ G_{JPA}(N_s + N_{int}) + (G_{JPA} - 1)N_i \right] \quad (14)$$

with  $N_s$  and  $N_i$  given by Eq.13 at frequency  $f_s$  and  $f_i$  respectively. For each frequency, we fitted the measured noise power with respect to  $V$  with Eq.14 and four fitting parameters:  $V_{shift}$ ,  $T$ ,  $G_{JPA}$  and  $N_{int}$ .  $G_{chain}$  is not a fitting parameter because it can be obtained by a noise measurement going through the 50  $\Omega$  PCB instead of the JPA with the same fitting method (with  $G_{JPA} = 1$  and  $G_{chain}$  a fitting parameter). We emphasize here that we did not take into account the losses between the SNTJ, the JPA and the HEMT to extract the different parameters. This makes the fitted gains smaller than the real values and the fitted intrinsic noise higher than the real value. This way the value we determine for the added noise is an upper bound.

### B. Effect of the saturation of the JPA

We saw in the main text that the 1 dB compression point is around -123 dBm. The SNTJ can thus saturate the JPA even at relatively low bias voltage because it is a broadband photon emitter. Experimentally, we sweep the bias voltage  $V$  between -400 and 400  $\mu$ V, but we see in the high gain region a saturation outside the range of -125 to 185  $\mu$ V. Thus, to fit  $T$ ,  $G_{JPA}$  and  $N_{int}$  we restrict the data to this range. This reduces the precision of the extracted  $N_{int}$ .

### C. Extracting $V_{shift}$

In order to get  $V_{shift}$ , in a first iteration, we fix  $T$  at 150 mK (close to the experimental one) and fit the PSD with Eq.14 for each frequency. We take the most probable value. From this we get  $V_{shift} = 31.55 \mu$ V. Fig. S8 shows such a fit for a frequency of 6.143 GHz.

### D. Extracting $T$

The electronic temperature is a very important parameter especially when  $N_{int}$  is close to the quantum limit. To have an estimation of  $T$ , we fitted the PSD obtained by the noise measurement on the 50  $\Omega$  PCB instead of the JPA (Fig. S1a) and

obtained  $T \approx 160$  mK. Fitting  $T$  directly with a noise measurement on the JPA gives  $T \approx 210$  mK but is less accurate because of the saturation effect limiting the bias voltage range available for the fit. The value of the electronic temperature depends on DC filtering and grounding of the SNTJ and it is not surprising that it largely exceeds the base temperature of the dilution fridge. We chose to keep  $T = 160$  mK because it also overestimates the fitted added noise compared to  $T = 210$  mK.

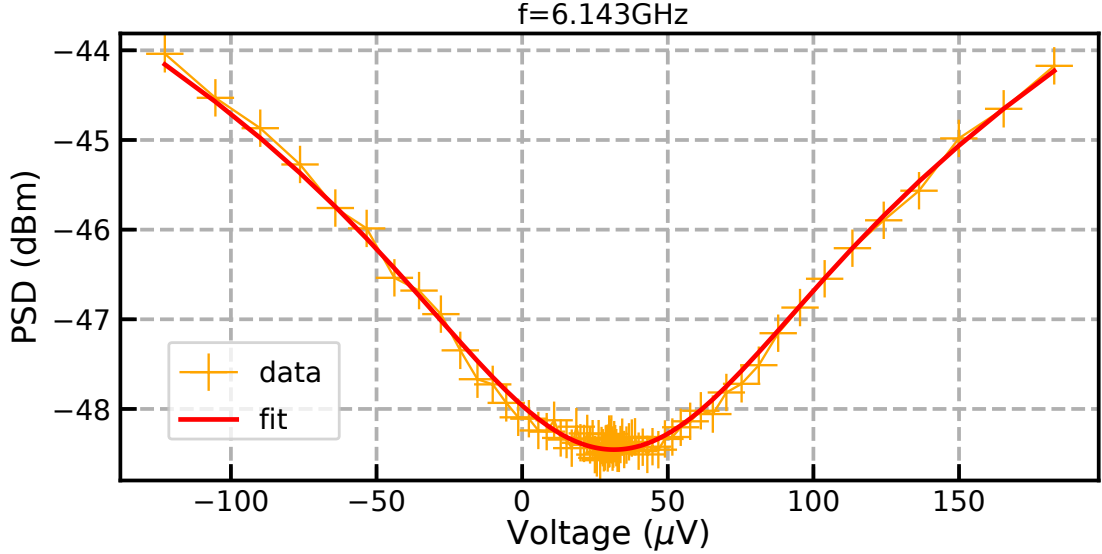

Figure S8: PSD as a function of the voltage biasing the SNTJ at  $f=6.143$  GHz.

#### E. Extracting $G_{JPA}$ and $N_{int}$

Once the electronic temperature  $T$  is fixed, we perform a last fit of the PSD with only two parameters:  $G_{JPA}$  and  $N_{int}$ . We have thus an additional way of controlling the fit quality by comparing the fitted gain from the PSD measurement with the experimental gain obtained from a direct VNA measurement. We also compute the deviation between the fit and the measured data. If the deviation is above a fixed threshold we do not take the fitted noise and gain into account. Close to the pump frequency, the measured signal is perturbed by the strong pump tone because of the 2 MHz bandwidth of the spectrum analyzer. This explains the missing central data points in Fig. 4b and 4c of the main text.

During the fitting process we do not take into account the losses between the SNTJ and the JPA (estimated to 2-3 dB at maximum). This makes the value of the extracted

system noise larger than the reality. If there is  $\alpha$  dB of loss, the true intrinsic noise is  $N_{int}/10^{\frac{\alpha}{10}}$ . Thus while there is some uncertainty on the exact noise value, our procedure ensures that we do not underestimate the noise of the JPA.

### F. Added noise for different gate voltages

We performed noise measurement for different gate voltages in order to see if the noise added by the amplifier is close to the quantum limit on the whole frequency range. This was not possible on the full range of frequencies for several experimental reasons. The first is the "charge instability" of the system, making the resonator frequency drifts during long measurements (see section III). It was thus difficult to maintain optimized parameters (pump frequency and power) during the whole noise measurement. Indeed, we see in Fig. S9a that for a different frequency the noise performance is not as good as the one presented in the main text. But this is explained by the low gain of the JPA (10 dB) in this experiment, as shown in Fig. S9b. This is not enough to overcome the added noise coming from the HEMT. This "charge instability" forced us to make quick measurements, thus lowering the precision. Moreover, working at lower frequencies (higher  $K$ ) made the ratio  $\gamma/K$  smaller and so, the saturation power of the JPA lower. Therefore, the bias voltage range of the SNTJ on which we fitted the PSD was very small, making the fit not as reliable. Nonetheless, we can clearly see in Fig. S9a,c and d, that the gate tunable graphene JPA dramatically improves the noise performance compared to the HEMT.

## VII. ADDITIONAL DEVICES

We measured a similar device with a gJJ width of  $2\ \mu\text{m}$ , a resonator width of  $5\ \mu\text{m}$  and less on-chip gate filtering. In Fig. S10a we plot the differential resistance  $dV/dI$  as a function of the bias current  $I_b$  and the gate voltage  $V_g$ . Close to  $V_g=-8\ \text{V}$  and  $V_g=6\ \text{V}$  the device exhibited current leakage through the gate. We were thus not able to reach the Dirac point. The critical current can be modulated from  $0.5\ \mu\text{A}$  to  $1.2\ \mu\text{A}$ . This enabled the control of the resonance frequency from  $5.8\ \text{GHz}$  to  $6.05\ \text{GHz}$  as we can see in Fig. S10b where the phase of the  $S_{11}$  parameter is plotted with respect to the gate voltage. The  $S_{11}$  parameter was here normalized with a trace taken at  $1.1\ \text{K}$  before the device entered in the superconducting state. In Fig. S10c the gain

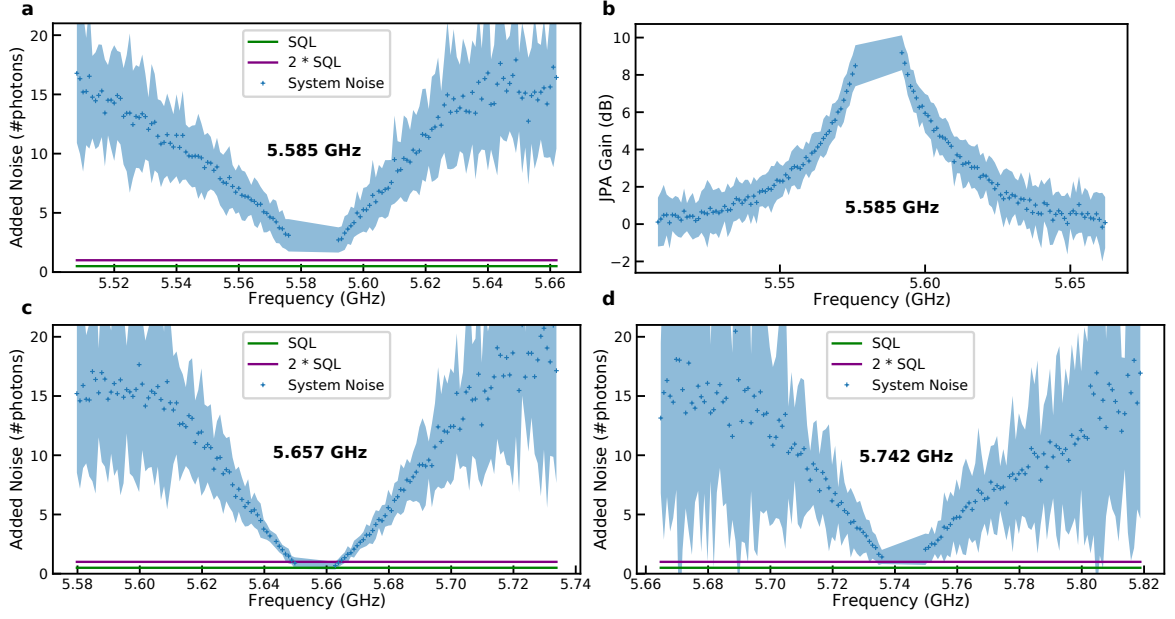

Figure S9: Noise analysis for different gate voltages. (a), (c) and (d): system noise fitted for different JPA working frequencies. (b) Gain extracted from the PSD measurement of the JPA working at 5.585 GHz.

of the graphene based JPA is plotted for three gate voltages (-7.2 V, -6.1 V, -3.5 V). The gain is above 15 dB on the full range of frequency reachable by the device. We also measured parametric amplification on another device which was not electrically tunable.

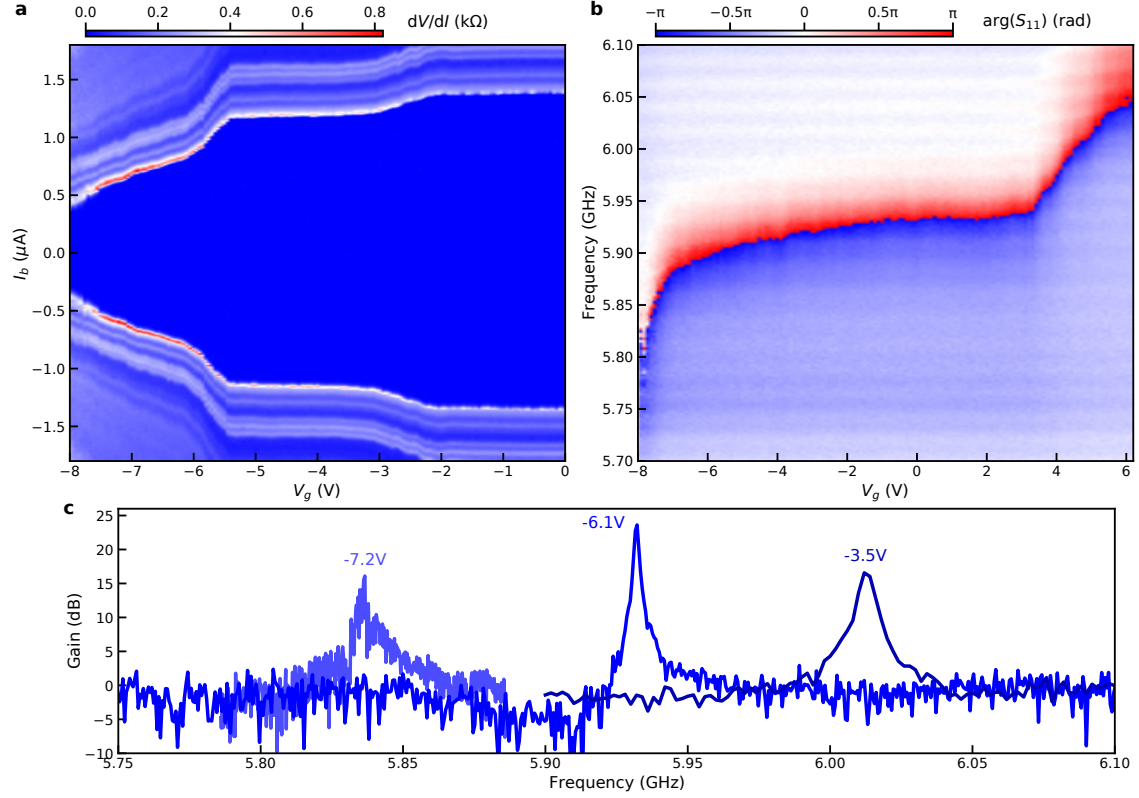

Figure S10: Additional device measurement. (a) Differential resistance as a function of the bias current and gate voltage. (b)  $S_{11}$  as a function of gate voltage. (c) Gain measured for three different gate voltages.

- 
- [1] S. Probst, F. B. Song, P. A. Bushev, A. V. Ustinov, and M. Weides, Efficient and robust analysis of complex scattering data under noise in microwave resonators, [Review of Scientific Instruments](#) **86**, 16 (2015), [arXiv:1410.3365](#).
  - [2] F. E. Schmidt, M. D. Jenkins, K. Watanabe, T. Taniguchi, and G. A. Steele, A ballistic graphene superconducting microwave circuit, [Nature Communications](#) **9**, 1 (2018), [arXiv:1806.11389](#).
  - [3] M. Titov, A. Ossipov, and C. W. Beenakker, Excitation gap of a graphene channel with superconducting boundaries, [Physical Review B - Condensed Matter and Materials Physics](#) **75**, 1 (2007), [arXiv:0609623 \[cond-mat\]](#).
  - [4] T. Klapwijk, G. Blonder, and M. Tinkham, Explanation of subharmonic energy gap structure in superconducting contacts, [Physica B+C](#) **109-110**, 1657 (1982).

- 
- [5] J. Park, J. H. Lee, G. H. Lee, Y. Takane, K. I. Imura, T. Taniguchi, K. Watanabe, and H. J. Lee, Short Ballistic Josephson Coupling in Planar Graphene Junctions with Inhomogeneous Carrier Doping, [Physical Review Letters](#) **120**, 77701 (2018).
- [6] B. Yurke and E. Buks, Performance of cavity-parametric amplifiers, employing Kerr nonlinearities, in the presence of two-photon loss, [Journal of Lightwave Technology](#) **24**, 5054 (2006), [arXiv:0505018 \[quant-ph\]](#).
- [7] B. A. Kochetov and A. Fedorov, Higher-order nonlinear effects in a Josephson parametric amplifier, [Physical Review B - Condensed Matter and Materials Physics](#) **92**, 1 (2015), [arXiv:1509.06154](#).
- [8] M. Malnou, M. Vissers, J. Wheeler, J. Aumentado, J. Hubmayr, J. Ullom, and J. Gao, Three-Wave Mixing Kinetic Inductance Traveling-Wave Amplifier with Near-Quantum-Limited Noise Performance, [PRX Quantum](#) **2**, 010302 (2021), [arXiv:2007.00638](#).
- [9] A. Ranadive, M. Esposito, L. Planat, E. Bonet, C. Naud, O. Buisson, W. Guichard, and N. Roch, [A reversed Kerr traveling wave parametric amplifier](#) (2021), [arXiv:2101.05815](#).
